# Supplementary material for: PrivacyProber: Assessment and Detection of Soft-Biometric Privacy-Enhancing Techniques
Source: arXiv:2211.08864 source file (2022-11-22)
Supplement: Supplementary file 1 [file appendix.tex]

\begin{appendices}

\section{}
In this section we present some additional information on the procedures proposed and implemented in the paper with the goal of facilitating reproducibility. We also present additional results to further highlight the merits of the proposed PrivacyProber and the PD$^2$ privacy enhancement detection technique.

\subsection{Implementational Details}
In the main part of the paper, we presented several possibilities for implementing the proposed PrivacyProber and briefly introduced the considered privacy models. While the main concepts have been elaborated on, in depth implementational details were omitted for brevity. Here we provide additional information to help with the reproducibility of the paper.

\subsubsection{Implementing the Inpainting Procedure}
The inpainting procedure, $\chi_{in}$, described in Section~\ref{SubSubSec: Inpainting}, relies on a chess--like pattern to mask out regions for inpainting. The pattern used in this work was designed based on $36$ square regions of size $5 \times 5$ pixel, with $30$ pixels between the squares. The pattern is shifted by $1$ pixel in the horizontal and vertical direction to produce a total of $N=1,156$ binary masks that are then used for inpainting. These values and concrete appearance of the pattern were selected based on preliminary experiments and manual inspection of the inpainting quality. No special effort was made to optimize the pattern for optimal attribute recovery, which is a particularly strong observation given the success of the inpainting procedure in the experimental evaluation.   

We also note that the proposed procedure is not limited only to the chess--like pattern used in this work. Any masking pattern that offers a reasonable trade--off between the size of the masked regions and contextual information left intact should provide comparable results. Additionally, the procedure is agnostic with respect to the inpainting model utilized and can, therefore, benefit from future advances in this area image inpainting.

\subsubsection{Implementing the Super--Resolution Procedure}

For the super--resolution--based attribute recovery procedure, $\chi_{sr}$, described in Section~\ref{SubSubSec: Inpainting} %, we use a Gaussian kernel $g$ of size $X \time X$ pixel and standard deviation of $\sigma = X$ for smoothing. W
we downscale images by a factor of $s=3.6$ using bilinear interpolation. Thus, we resize images from the original size of $224\times 224$ to $64\times 64$ pixels before applying super--resolution to upscale the images to the original resolution. %These values were set, so as to avoid aliasing effects and to ensure that a the high--frequency information removed during downscaling could be recovered to a reasonable extent with the super--resolution model. 
Again, no special effort was made to optimize the downsampling factor of this procedure for better performance, instead a few sample images were manually examined for the visual quality of the super--resolved images. %As we have shown in the experimental section of the main paper, the procedure still ensured   

\subsubsection{Implementing the privacy models}

We use three different soft--biometric privacy models in our experiments, $k$--AAP, FGSM and FlowSAN (FlowSAN--3 and FlowSAN--5). Table~\ref{tab: model params} provide technical details about the hyper--parameters used in the experiments.
\begin{table}[!tb]
\centering
\caption{Parameter settings used to implement the considered privacy models.}

\label{tab: model params}
\resizebox{\columnwidth}{!}{%
\begin{tabular}{lrrr} \hline\hline
Model & Strategy & Parameters \\
\hline
$k$--APP & Fixed parameters & \#max iter.: 20, Learn. rate: 0.01, Init. const.: 1,000 \\
FGSM & Value search & Range: [0.9 -- 0.51],    \#Epochs: 200, Epsilon: 0.5 \\%Resolution: XX \\
FlowSAN & Two versions & \#SANs in sequence: 3 and 5\\
\hline \hline \vspace{-2mm}
\end{tabular}}
\end{table}

\subsection{Combined tampering Detection}

In the main part of the paper we showed that our learning--free PD$^2$ tampering  detection approach was able to detect  privacy enhancement in facial images with high accuracy. This was done without considering tampered examples for learning, as needed by competing techniques, such as the state--of--the-art T--SVM detection approach from~\cite{agarwal2020image}. PD$^2$ was demonstrated to outperform T--SVM, but as observed in the qualitative analysis, made detection mistakes with images of poor quality and obvious artifacts, where the performance of the supervised T--SVM approach  is the strongest. To consider the best of both worlds, we explore in this section a combination of the two detection approaches. 
To make the experimental setup as challenging as possible, we again assume a black box scenario for T--SVM (denoted as T--SVM (A) in Section~\ref{SubSEc: PD comparison} and Table~\ref{tab: detection combination}) and train it on FlowSAN--5 enhanced images from LFW. We then use this model with all remaining (unseen) privacy models and all experimental datasets, similarly to PD$^2$. 

Given an input face image $I$, both PD$^2$ and T--SVM generate a tampering score, $s_{pd2}(I)$ and $s_{tsvm}(I)$, that can be used to flag privacy enhanced images. Because the two detection techniques represent independent data sources, we combine the two scores using a weighted product fusion rule, i.e.:
\begin{equation}
    s = s_{pd2}^{\alpha}\cdot s_{tsvm}^{1-\alpha},
\end{equation}
or equivalently in the log domain, which better highlights the impact of the balancing factor $\alpha$
\begin{equation}
    \log(s) = \alpha\log(s_{pd2})+(1-\alpha)\log(s_{tsvm}).
\end{equation}
In the above equations $s$ denotes the combined tampering score and the dependence on $I$ is omitted for better readability. The balancing factor is set to $\alpha=0.5$ to consider both models equally during detection. %Note also that with the above fusion rule no prior score normalization is needed. 
\begin{table}[!tb]
\centering
\caption{AUC scores ($\mu\pm\sigma$) for privacy-enhancement detection experiments. The learning-free (black box) PD$^2$ approach is combined with the classification--based T--SVM techniques from~\cite{agarwal2020image} trained in a black box scenario. The combined approach offers competitive performance across all datasets and privacy models, pointing to the complementarity of the two detection approaches.}

\label{tab: detection combination}
\resizebox{\columnwidth}{!}{%
\footnotesize
\begin{tabular}{lrrcc} \hline\hline
\multirow{2}{*}{Privacy Model} & \multirow{2}{*}{Dataset}  & \multirow{ 2}{*}{PD$^2$ (ours)}  & \multicolumn{1}{c}{Black box} & \multirow{ 2}{*}{Combined (ours)}\\ 
\cline{4-4} 
         && & T--SVM (A)$^\dagger$  &  \\\hline
\multirow{ 3}{*}{$k$--AAP}  & LFW  &   
$0.980 \pm 0.003$ & $0.743\pm 0.013$  &  $0.952\pm 0.016$ \\
                            & MUCT & 
$0.984 \pm 0.001$  & $0.727\pm 0.030$   &  $0.966\pm 0.009$\\
                            & Adience  & 
$0.828 \pm 0.002$  & $0.604\pm 0.008$  &  $0.715\pm 0.011$        \\
                            \arrayrulecolor{gray}\hline
\multirow{ 3}{*}{FGSM} & LFW  & 
$0.992 \pm 0.001$  & $0.894\pm 0.013$  &  $0.990\pm 0.005$\\
                            & MUCT & 
$0.995 \pm 0.000$  & $0.858\pm 0.015$  &  $0.987\pm 0.004$ \\
                            & Adience  &  
$0.877 \pm 0.004$  & $0.595\pm 0.016$  &  $0.738\pm 0.017$ \\
\arrayrulecolor{gray}\hline

\multirow{ 2}{*}{FlowSAN--3} & LFW  & 
$0.980 \pm 0.002$  & $1.000\pm 0.000$  &  $1.000\pm 0.000$ \\
                            & MUCT & 
$0.991 \pm 0.003$ & $1.000\pm 0.000$  &  $1.000\pm 0.000$ \\
                            & Adience  &  
$0.696 \pm 0.003$  & $1.000\pm 0.000$  &  $1.000\pm 0.000$ \\
\arrayrulecolor{gray}\hline
\multirow{ 2}{*}{FlowSAN--5} & LFW  & 
$0.976 \pm 0.002$  & $1.000\pm 0.000$ &  $1.000\pm 0.000$  \\
                            & MUCT &
$0.991 \pm 0.004$  & $1.000\pm 0.000$  &  $1.000\pm 0.000$ \\
                            & Adience & 
$0.751 \pm 0.003$  & $1.000\pm 0.000$ &  $1.000\pm 0.000$  \\
\arrayrulecolor{black}
\hline \hline
\multicolumn{5}{l}{\scriptsize $^\dagger$ Detection model trained on FlowSAN--5 and LFW.}
\end{tabular}%\vspace{-2.5mm}
}
\end{table}

We run experiments using the same setup as in Section~\ref{SubSEc: PD comparison} and report results in Table~\ref{tab: detection combination}. As can be seen, the combined approach achieves comparable detection performance to PD$^2$ for $k$--AAP and FGSM on LFW and MUCT. On these datasets, PD$^2$ clearly outperformed T--SVM and this performance is also reflected in the combination of the two models. For privacy enhancement with the FlowSAN models, the combination of the detection techniques again performs equivavlently to the better performing of the two individual models on all experimental datasets. Here, the combined detection approach achieves ideal performance with an AUC score of $1$ and further improves on the initial performance of the PD$^2$ technique, which was the weaker of the two detection models on this dataset. %A considerable performance jump is observed on the Adience dataset, where PD$^2$ on its own results in mean AUC scores of $0.696$ and $0.751$ with FlowSAN--3 and FlowSAN--5 tampered images, respectively, the combined approach, on the other hand, achieves ideal AUC scores of 1. 
We do also observe a performance degradation with the combined approach compared to the better performing individual model. Specifically, for the $k$--AAP and FGSM privacy enhanced images from the Adience dataset. However, this degradation is smaller than the performance gain we observe with the FlowSAN models on the same dataset, the combined approach outperforms T--SVM, but generates weaker AUC scores than PD$^2$.   

Overall, the experimental results suggest that the combination of PD$^2$ and  is beneficial for the detecting privacy enhancement and contributes towards more robust performance across different privacy models and data characteristics. The conceptual differences between PD$^2$ and T--SVM allow the combined approach to capture complementary information for the detection procedure in produce more reliable tempereing scores across all experiments.        

\end{appendices}
